# Supplementary material for: Modeling streamer discharges as advancing imperfect conductors
Source: arXiv:1705.03276 source file (2017-05-09)
Supplement: Supplementary file 1 [file sausageSupp.pdf]

# Chemical model for the article *Modeling streamer discharges as advancing imperfect conductors*

May 9, 2017

The chemical model of this article was implemented using CHEMISE (CHEMical System Evaluator)[a]. The table in the following page has been produced automatically using CHEMISE's LaTeX-export feature.

Note that besides abundant neutrals $O_2$, $N_2$ and $H_2O$ our model includes only ion species. Therefore we do not consider the product species in recombination reactions 24 and 25. Note also that in rection 25 $A^+$ and $B^-$ are placeholders for any positive and negative ions, respectively. Thus that reaction encompasses 54 actual reactions.

The rates for reactions denoted as $f(E/n)$ are calculated from Bolsig+ [Hagelaar and Pitchford, 2005] using the cross-section data from [Phelps and Pitchford, 1985] retrieved from the LxCat web [Pancheshnyi et al., 2012] [b].

In the table all magnitudes are in SI unitex except $E/n$, which is expressed in Townsend ($1\,\mathrm{Td} = 10^{-21}\,\mathrm{Vm}^2$). The ion temperature $T_i$ is calculated as $T_i = T + \frac{1}{g}\frac{E}{n}$ with $g = 0.18\,\mathrm{Td\,K}^{-1}$ [Gallimberti, 1979].

[a] Source code and a short introduction are accessible at `https://gitlab.com/aluque/chemise`.

[b] `https://lxcat.net`

| | Reaction | | Rate ($m^{3(n-1)}s^{-1}$) | Reference |
|---|---|---|---|---|
| **1** | $e + N_2$ | $\longrightarrow 2e + N_2^+$ | $f(E/n)$ | |
| **2** | $e + O_2$ | $\longrightarrow 2e + O_2^+$ | $f(E/n)$ | |
| **3** | $e + O_2 + O_2$ | $\longrightarrow O_2^- + O_2$ | $f(E/n)$ | |
| **4** | $e + O_2$ | $\longrightarrow O + O^-$ | $f(E/n)$ | |
| **5** | $M + O_2^-$ | $\longrightarrow e + O_2 + M$ | $k_0 e^{-\left(\frac{a}{b+E/n}\right)^2}$ [$k_0 = 1.24 \times 10^{-17}$, $a = 179$, $b = 8.8$] | [Pancheshnyi, 2013] |
| **6** | $O_2 + O^-$ | $\longrightarrow O_2^- + O$ | $k_0 e^{-\left(\frac{a}{b+E/n}\right)^2}$ [$k_0 = 6.96 \times 10^{-17}$, $a = 198$, $b = 5.6$] | [Pancheshnyi, 2013] |
| **7** | $N_2 + O^-$ | $\longrightarrow e + N_2O$ | $k_0 e^{-\left(\frac{a}{b+E/n}\right)^2}$ [$k_0 = 1.16 \times 10^{-18}$, $a = 48.9$, $b = 11$] | [Pancheshnyi, 2013] |
| **8** | $O_2 + O^- + M$ | $\longrightarrow O_3^- + M$ | $k_0 e^{-\left(\frac{E/n}{a}\right)^2}$ [$k_0 = 1.1 \times 10^{-42}$, $a = 65$] | [Pancheshnyi, 2013] |
| **9** | $O_2^- + H_2O + M$ | $\longrightarrow O_2^- \cdot (H_2O) + M$ | $2.2 \times 10^{-40}$ | [Gallimberti, 1979] |
| **10** | $O_2^- \cdot (H_2O) + M$ | $\longrightarrow O_2^- + H_2O + M$ | $k_0 e^{\left(\frac{\Delta G}{kT_i}\right)}$ [$k_0 = 5.91 \times 10^{-15}$, $\Delta G = -1.28 \times 10^{-19}$] | [Gallimberti, 1979] |
| **11** | $O_2^- \cdot (H_2O) + H_2O + M$ | $\longrightarrow O_2^- \cdot (H_2O)_2 + M$ | $5 \times 10^{-40}$ | [Gallimberti, 1979] |
| **12** | $O_2^- \cdot (H_2O)_2 + M$ | $\longrightarrow O_2^- \cdot (H_2O) + H_2O + M$ | $k_0 e^{\left(\frac{\Delta G}{kT_i}\right)}$ [$k_0 = 1.34 \times 10^{-14}$, $\Delta G = -5.8 \times 10^{-20}$] | [Gallimberti, 1979] |
| **13** | $O_2^- \cdot (H_2O)_2 + H_2O + M$ | $\longrightarrow O_2^- \cdot (H_2O)_3 + M$ | $5 \times 10^{-41}$ | [Gallimberti, 1979] |
| **14** | $O_2^- \cdot (H_2O)_3 + M$ | $\longrightarrow O_2^- \cdot (H_2O)_2 + H_2O + M$ | $k_0 e^{\left(\frac{\Delta G}{kT_i}\right)}$ [$k_0 = 1.34 \times 10^{-15}$, $\Delta G = -4.49 \times 10^{-20}$] | [Gallimberti, 1979] |
| **15** | $N_2^+ + N_2 + M$ | $\longrightarrow N_4^+ + M$ | $5 \times 10^{-41} \times (300/T)^3$ | [Aleksandrov and Bazelyan, 1999] |
| **16** | $N_4^+ + O_2$ | $\longrightarrow 2N_2 + O_2^+$ | $2.5 \times 10^{-16} \times (300/T)^3$ | [Aleksandrov and Bazelyan, 1999] |
| **17** | $O_2^+ + O_2 + M$ | $\longrightarrow O_4^+ + M$ | $2.4 \times 10^{-42} \times (300/T)^3$ | [Aleksandrov and Bazelyan, 1999] |
| **18** | $O_2^+ + H_2O + M$ | $\longrightarrow O_2^+ \cdot (H_2O) + M$ | $2.6 \times 10^{-40}$ | [Aleksandrov and Bazelyan, 1999] |
| **19** | $O_2^+ \cdot (H_2O) + H_2O$ | $\longrightarrow H_3O^+ + OH + O_2$ | $3 \times 10^{-16}$ | [Aleksandrov and Bazelyan, 1999] |
| **20** | $H_3O^+ + H_2O + M$ | $\longrightarrow H_3O^+ \cdot (H_2O) + M$ | $3 \times 10^{-39}$ | [Aleksandrov and Bazelyan, 1999] |
| **21** | $H_3O^+ \cdot (H_2O) + H_2O + M$ | $\longrightarrow H_3O^+ \cdot (H_2O)_2 + M$ | $3 \times 10^{-39}$ | [Aleksandrov and Bazelyan, 1999] |
| **22** | $H_3O^+ \cdot (H_2O)_2 + H_2O + M$ | $\longrightarrow H_3O^+ \cdot (H_2O)_3 + M$ | $3 \times 10^{-39}$ | [Aleksandrov and Bazelyan, 1999] |
| **23** | $e + H_3O^+ \cdot (H_2O)_3$ | $\longrightarrow H + 4H_2O$ | $6.5 \times 10^{-12} \times (300/T_e)^{0.5}$ | [Aleksandrov and Bazelyan, 1999] |
| **24** | $e + O_4^+$ | $\longrightarrow$ | $f(E/n)$ | |

| | | | | |
|---|---|---|---|---|
| **25** | $A^+ + B^-$ | $\longrightarrow$ | $1 \times 10^{-13}$ | [Kossyi et al., 1992] |

## 0.1 Mobilities

| **Species** | **Reduced mobility** ($m^{-1}V^{-1}s^{-1}$) | **Reference** |
|---|---|---|
| $O_2{}^-$ | $7.1 \times 10^{21}$ | |
| $H_3O^+$ | $5.4 \times 10^{21}$ | |
| $O^-$ | $1.2 \times 10^{22}$ | |
| e | $1 \times 10^{24}$ | |
| $O_2{}^+$ | $5.4 \times 10^{21}$ | |
| $O_2{}^- \cdot (H_2O)_2$ | $5.4 \times 10^{21}$ | |
| $H_3O^+ \cdot (H_2O)_3$ | $5.4 \times 10^{21}$ | |
| $N_2{}^+$ | $5.4 \times 10^{21}$ | |
| $O_2{}^- \cdot (H_2O)_3$ | $5.4 \times 10^{21}$ | |
| $O_4{}^+$ | $5.4 \times 10^{21}$ | |
| $O_3{}^-$ | $7.6 \times 10^{21}$ | |
| $O_2{}^- \cdot (H_2O)$ | $5.4 \times 10^{21}$ | |
| $H_3O^+ \cdot (H_2O)_2$ | $5.4 \times 10^{21}$ | |
| $N_4{}^+$ | $5.4 \times 10^{21}$ | |
| $H_3O^+ \cdot (H_2O)$ | $5.4 \times 10^{21}$ | |
| $O_2{}^+ \cdot (H_2O)$ | $5.4 \times 10^{21}$ | |

# References


[Aleksandrov and Bazelyan, 1999] Aleksandrov, N. L. and Bazelyan, E. M. (1999). Ionization processes in spark discharge plasmas. *Plasma Sour. Sci. Technol.*, 8:285.

[Gallimberti, 1979] Gallimberti, I. (1979). The mechanism of the long spark formation. *Journal de Physique*, 40:193.

[Hagelaar and Pitchford, 2005] Hagelaar, G. J. M. and Pitchford, L. C. (2005). Solving the Boltzmann equation to obtain electron transport coefficients and rate coefficients for fluid models. *Plasma Sour. Sci. Technol.*, 14:722.

[Kossyi et al., 1992] Kossyi, I. A., Kostinsky, A. Y., Matveyev, A. A., and Silakov, V. P. (1992). Kinetic scheme of the non-equilibrium discharge in nitrogen-oxygen mixtures. *Plasma Sour. Sci. Technol.*, 1:207.

[Pancheshnyi, 2013] Pancheshnyi, S. (2013). Effective ionization rate in nitrogen-oxygen mixtures. *J. Phys. D*, 46(15):155201.

[Pancheshnyi et al., 2012] Pancheshnyi, S., Biagi, S., Bordage, M. C., Hagelaar, G. J. M., Morgan, W. L., Phelps, A. V., and Pitchford, L. C. (2012). The LXCat project: Electron scattering cross sections and swarm parameters for low temperature plasma modeling. *Chem. Phys.*, 398:148.

[Phelps and Pitchford, 1985] Phelps, A. V. and Pitchford, L. C. (1985). Anisotropic scattering of electrons by N2 and its effect on electron transport. *Phys. Rev. A*, 31:2932.
